# Supplementary material for: Quantum interference of topological states of light
Source: arXiv:1904.10612 source file (2019-04-24)
Supplement: Supplementary file 1 [file supp.pdf]

# Supplementary Materials for Quantum interference of topological states of light

Jean-Luc Tambasco[1], Giacomo Corrielli[2, 3], Robert J. Chapman[1], Andrea Crespi[2, 3], Oded Zilberberg[4], Roberto Osellame[2, 3], and Alberto Peruzzo[1]

[1] *Quantum Photonics Laboratory and Centre for Quantum Computation and Communication Technology, School of Engineering, RMIT University, Melbourne, Victoria 3000, Australia*

[2] *Istituto di Fotonica e Nanotecnologie, Consiglio Nazionale delle Ricerche, Piazza Leonardo da Vinci 32, Milano I-20133, Italy*

[3] *Dipartimento di Fisica, Politecnico di Milano, Piazza Leonardo da Vinci 32, Milano I-20133, Italy*

[4] *Institute for Theoretical Physics, ETH Zurich, 8093 Zurich, Switzerland*

August 5, 2018

# Overview

S1. Experimental Setup

S2. SPDC Source

S3. HOM Dip

# S1 Experimental Setup

For classical characterization, we use an optical fiber aligned to the input waveguides and ensure the fiber is positioned to excite the even mode across the two waveguides. The output is imaged with a CCD camera and telescope setup, focused onto the output face of the chip to clearly resolve the individual waveguides.

In order to couple a single photon into both boundary-states simultaneously, we use a v-groove fiber array with pitch of 127 $\mu$m and free-space optics to focus the photons onto the input waveguides. The input modes are separated by 80 $\mu$m and we use a two-lens setup to control the separation of the two photons. Figure S1 shows a ray-tracing schematic of the coupling setup. The lenses have 11 mm focal length and the spot size is kept large enough to illuminate both waveguides at each side of the array. Again, we ensure we excite the even mode at the input. Using both manual and automated optimization, we position the chip, free-space optics and fiber arrays such that we achieve maximum transmission through the chip. The coupling efficiency could be increased significantly by integrating onto the waveguide array a component that excites the symmetric supermode. This would enable coupling with a single optical fiber for each input and thus remove the majority of the coupling losses.

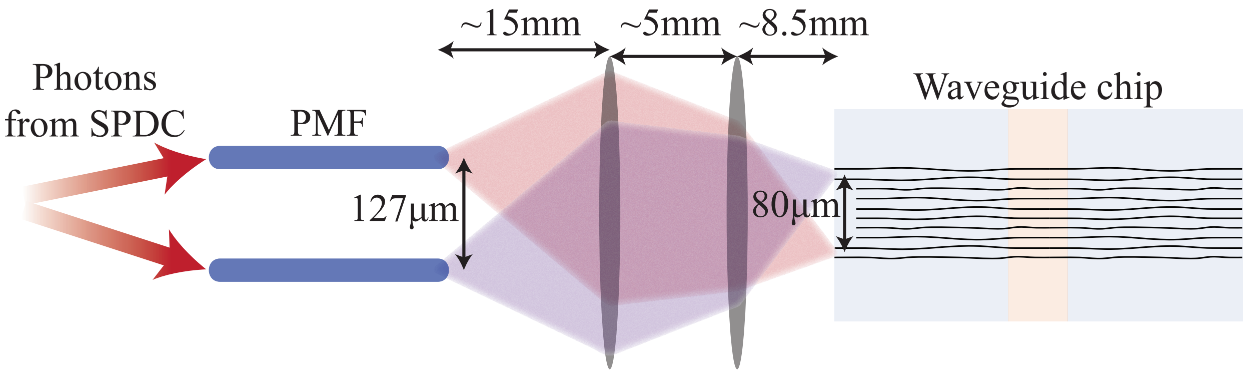


Figure S1: **Ray tracing simulation of the coupling setup.** The two photons are coupled out from polarization maintaining fiber (PMF) that are separated by 127 $\mu$m. Using two lenses, we focus the two photons into the chip with a separation of 80 $\mu$m.

## S2 SPDC Source

Horizontally polarized photon pairs at 807.5 nm are generated via type 1 spontaneous parametric down conversion (SPDC) in a 1 mm thick BiBO crystal, pumped by an 80 mW, 403.75 nm CW diode laser. The generated photons have an opening angle of 3° which enables easy extraction from the pump beam. The photons are passed through 3.1 nm narrow band filters before collection into polarization maintaining optical fiber. One fiber is mounted on a motorized stage to enable a tunable delay of up to 25 mm. Single photons are detected in coincidence using silicon avalanche photo-diodes. To reduce noise we subtract accidental counts by measuring uncorrelated two photon events with an applied electronic delay on one channel.

## S3 HOM Dip

The HOM interference was chosen as a means to verify the TBS as a quantum operation; specifically, a Hadamard gate. However, the quality of the HOM interference is limited by noise and imperfections in the device.

The error in the HOM dip visibility is calculated as

$$\epsilon_V = \frac{min(\mathbf{d})}{max(\mathbf{d})}\sqrt{\frac{1}{max(\mathbf{d})} + \frac{1}{min(\mathbf{d})}}, \quad \text{(S1)}$$

where $\mathbf{d}$ are the data points in the HOM dip.

The HOM dip in fig. 4 of the main text approaches 0 but does not reach this value exactly is the distinguishability of the two photons and the non-ideal reflectivity ($R \neq 50\%$) of the beamsplitter. The HOM dip visibility is maximal only for $R = 50\%$. As reported in the manuscript, the SPDC source of photon pairs was independently tested using a high-quality fiber-coupled commercial beamsplitter (FBS) with measured $R = 49.0 \pm 0.1\%$, and resulted in $V = 94.5 \pm 0.5\%$. The non-unit visibility is due to polarization and wavelength mismatches, as well as coupling losses leading to accidental coincidences. All these effects contribute to the non-zero minimum in the dip.

The relative visibility achieved by the TBS with respect to the FBS is $V_{\text{relative}} = 98.5 \pm 3.5\%$. This discrepancy is attributed to imperfections in the device, including the mentioned non-ideal reflectivity and the limited signal-to-noise ratio due to non optimized coupling of the device. We conclude that if the source was to produce nearly perfectly indistinguishable photons, our TBS would create quantum interference with visibility close to $V \approx 98.5\%$. This very high value is the closest we can get to the ideal unitary visibility with the current signal-to-noise ratio.
